# Supplementary material for: An ideal Weyl semimetal induced by magnetic exchange
Source: arXiv:1901.10022 source file (2019-11-14)
Supplement: Supplementary file 1 [file CK5_EuCd2As2_Supplemental_Materials_JRS_7.pdf]

# Supplementary Information

## An ideal Weyl semimetal induced by magnetic exchange

**J.-R. Soh[1], F. de Juan[1,2,3], M. G. Vergniory[2,3], N. B. M. Schröter[4], M. C. Rahn[1,5], D. Y. Yan[6], J. Jiang[1,6,7], M. Bristow[1], P. A. Reiss[1], J. N. Blandy[8], Y. F. Guo[9,10], Y. G. Shi[6], T. K. Kim[11], A. McCollam[12], S. H. Simon[1],Y. Chen[1,9], A. I. Coldea[1] & A. T. Boothroyd[1,*]**

[1]Department of Physics, University of Oxford, Clarendon Laboratory, Oxford, OX1 3PU, UK. [2]Donostia International Physics Center, 20018 Donostia-San Sebastian, Spain. [3]IKERBASQUE, Basque Foundation for Science, Maria Diaz de Haro 3, 48013 Bilbao, Spain. [4]Paul Scherrer Institute, WSLA/202, 5232 Villigen PSI, Switzerland. [5]MPA-CMMS, Los Alamos National Laboratory, Los Alamos, New Mexico 87545, USA. [6]Beijing National Laboratory for Condensed Matter Physics, Institute of Physics, Chinese Academy of Sciences, Beijing 100190, China. [7]Advanced Light Source, Lawrence Berkeley National Laboratory, Berkeley, California 94720, USA. [8]Department of Chemistry, University of Oxford, Inorganic Chemistry Laboratory, Oxford, OX1 3QR, UK. [9]School of Physical Science and Technology, ShanghaiTech University, Shanghai 201210, China. [10]CAS Center for Excellence in Superconducting Electronics (CENSE), Shanghai 200050, China. [11]Diamond Light Source, Harwell Campus, Didcot, OX11 0DE, UK. [12]High Field Magnet Laboratory (HFML-EMFL), Radboud University, 6525 ED Nijmegen, Nijmegen, Netherlands. *e-mail: andrew.boothroyd@physics.ox.ac.uk

## 1. Sample characterisation

The crystal structure and crystallographic quality of the flux-grown $EuCd_2As_2$ (ECA) single crystals were checked on a 6-circle x-ray (Mo, $K_\alpha$) diffractometer (Oxford Diffraction). Figures S1a, b and c present the scattered intensities in the (HK0), (H0L) and (0KL) planes, respectively. Figures S1d, e and f are the corresponding calculated reciprocal space maps. The intensity distribution and the pattern of experimental Bragg peaks in panels a–c agree well with those in the calculated maps in panels d–f. Of the 956 detected Bragg reflections,

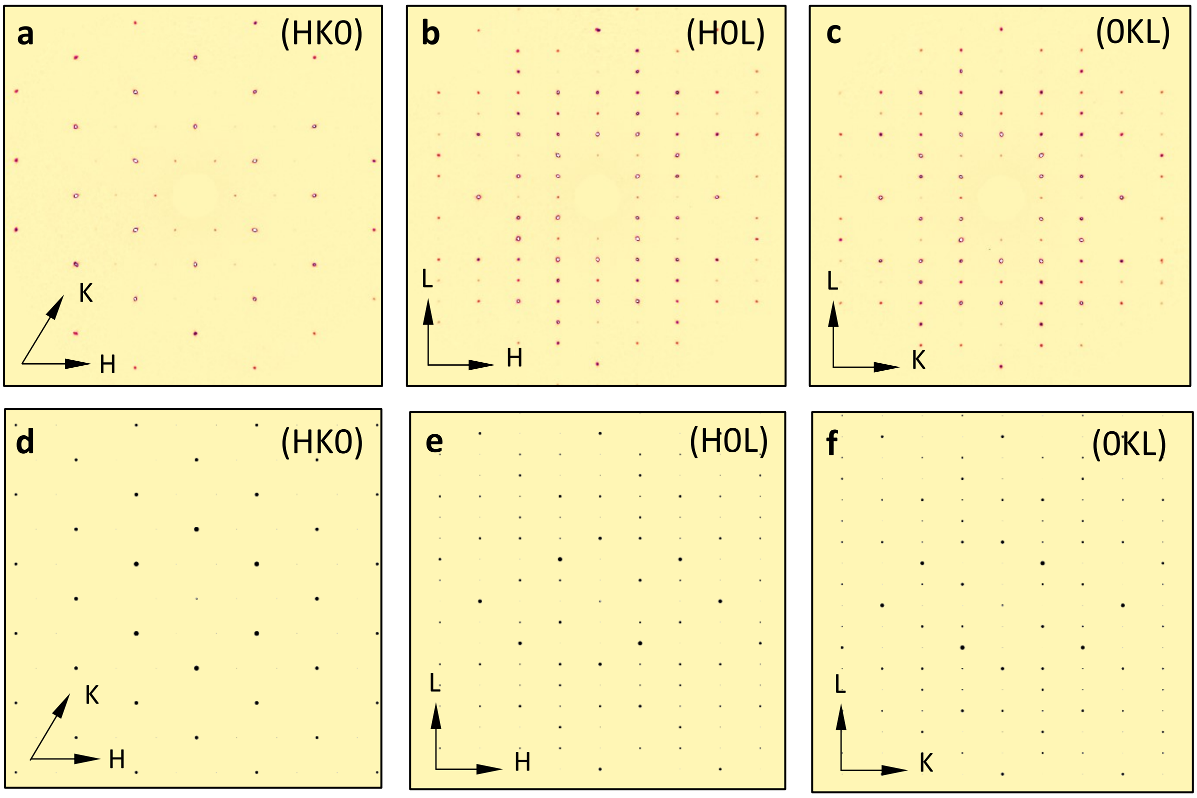


**Figures S1a–f. X-ray diffraction intensity maps in different reciprocal space planes for single crystalline ECA.**

98.7% fit with the P-3m1 space group (No. 164), in agreement with previous studies[1–4]. Moreover, the peaks display a very narrow mosaic, reflecting the good quality of the crystals. The flux-grown crystals have natural facets that reflect the underlying hexagonal symmetry, as shown in Figure S2. The direction of the corresponding crystal axes, *a*, *b* and *c*, was identified using a laboratory 6-circle X-ray diffractometer (Oxford Diffraction). The axes in Figure S2 correspond to that in the crystal structure in Figure 1a of the main article.

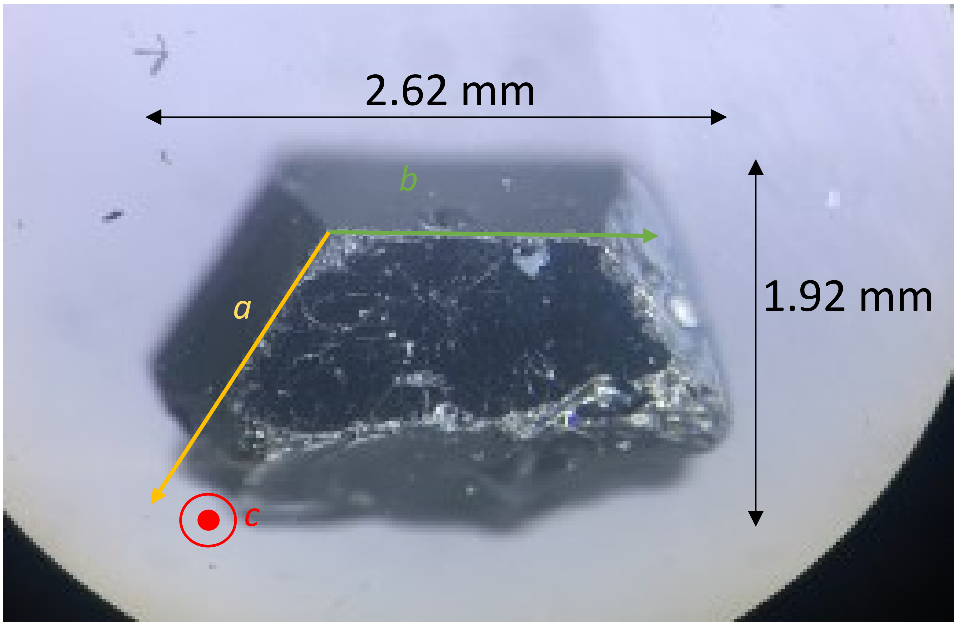


**Figure S2.** Image of a flux-grown crystal of dimensions ($2.62 \times 1.92 \times 1.25$ mm$^3$) with the corresponding crystal axes.

Magnetization measurements of single crystalline ECA were performed on a SQUID magnetometer (Quantum Design) at 2 K in fields up to 7 T. The curves in Figures S3a, b and c correspond to measurements in field directions **B**||**a**, **B**||**b*** and **B**||**c** respectively. In all field directions, the saturated moment is $M_{sat} \approx 7\ \mu_B$/f.u., which is consistent with the expected moment for fully divalent $Eu^{2+}$ ($4f^7$, $S = 7/2$ , $L = 0$). For **B**||**a** and **B**||**b***, the Eu moments fully saturate at B ≈ 0.8 T, whereas for **B**||**c**, the coercive field is ≈ 1.6 T. These results agree with the magnetometry measurements reported in Refs. 1–3.

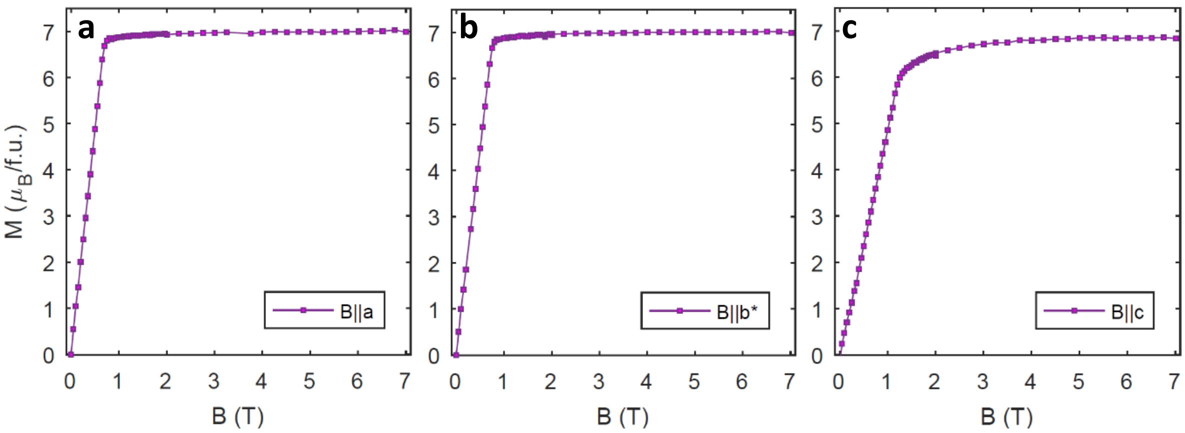


**Figure S3a–c. The magnetization data for single crystalline ECA at 2 K.**

For detailed structural analysis a small ECA crystal was cleaved and ground with an approximate 1:1 volume ratio of ground glass (in order to minimise absorption and preferred orientation effects). This powder was then loaded into a 0.5 mm diameter borosilicate capillary. The capillary was measured using synchrotron powder x-ray diffraction using the MAC detector on the I11 beamline at the Diamond Light Source, Didcot UK. The wavelength of the x-ray radiation was 0.824678 Å. The powder x-ray diffraction data was analysed by Rietveld refinement using TOPAS academic, version 5. [5]

The Rietveld plot of the powder diffraction data is shown in Figure S4. The sample was found to be ~99% pure hexagonal $EuCd_2As_2$. Two or three very small peaks are not indexed by the ECA model. These peaks most likely to arise from a small $Eu_xO_y$ or $Eu_xAs_y$ impurity (there are a few possible polymorphs). There is no trace of any $Cd_3As_2$ impurity phase. When allowed to vary, each of the atomic site occupancies converged to 100% within the error. Therefore, in the final fit the occupancies were fixed at 100%.

The refined structural parameters, listed in Table S1, are consistent with literature data[2].

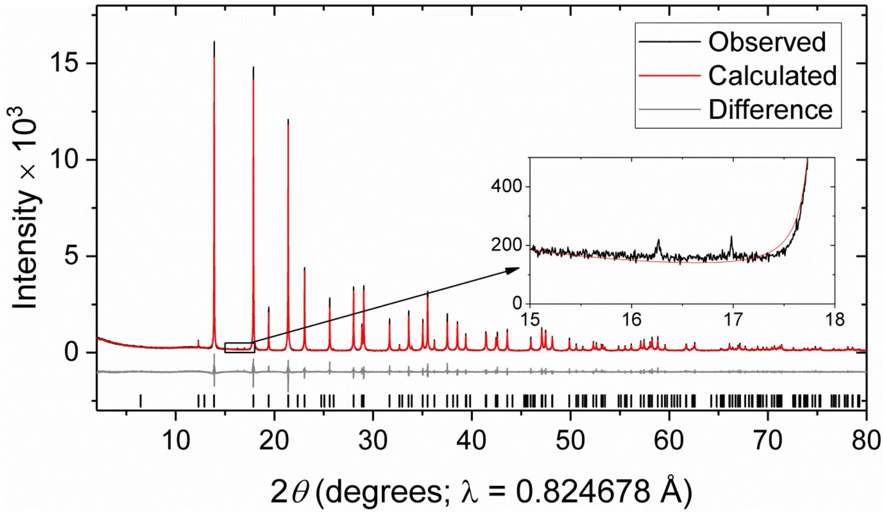


**Figure S4. Synchrotron x-ray powder diffraction pattern for ECA.** Rietveld plot of the ECA sample with inset to show the two largest peaks not indexed by the ECA phase**.** The x-ray powder diffraction data were collected at room temperature with the MAC detector on the I11 beamline.

**Table S1.** Structural parameters obtained from Rietveld refinement against powder x-ray diffraction data collected at room temperature using the MAC detector on the I11 beamline.

| Site | *x* | *y* | *z* | Occupancy | $U_{11}$ (Å$^2$) | $U_{22}$ (Å$^2$) | $U_{33}$ (Å$^2$) |
|---|---|---|---|---|---|---|---|
| Eu | 0 | 0 | 0 | 1* | 0.0147(8) | ≡$U_{11}$ | 0.0093(7) |
| Cd | ⅓ | ⅔ | 0.6332(1) | 1* | 0.0163(8) | ≡$U_{11}$ | 0.0136(9) |
| As | ⅓ | ⅔ | 0.2474(2) | 1* | 0.0116(8) | ≡$U_{11}$ | 0.0109(8) |
| $a$ = 4.44204(2) Å; $c$ = 7.33071(5) Å; Volume = 125.269(1) Å$^3$<br>Space group = $P$-3$m$1<br>$R_{wp}$ = 8.323%; $\chi^2$ = 1.767 | | | | | | | |

*not refined

# 2. High field magnetotransport

High-field magnetotransport measurements were performed using an ac four-probe technique at the High Field Magnet Laboratory (HFML) in Nijmegen (up to 37 T), and at the National High Magnetic Field Laboratory (NHMFL) in Tallahassee (up to 45 T). Figure S5a shows the in-plane resistivity measured on an as-grown single crystal with dimensions of 0.5x0.2x0.085 $mm^3$, at HFML at 1.4 K and in fields up to 37 T with **B||c**. The resistivity displays approximately 3 periods of Shubnikov–de Haas (SdH) quantum oscillations. To remove the magnetoresistance background and extract the information about the oscillatory spectrum, we (1) symmetrized the data as shown in Figure S5b, (2) took the first and second derivatives of the symmetrized data as shown in Figures S5c–d, (3) found the peaks and valleys of these oscillations, and (4) calculated the gradient of the slope of the Landau fan plot as shown in Figure 3d in the main article. Note, however, that if integers are assigned to the maxima rather than the minima in $\rho_{xx}$, as prescribed in Ref. 6, then the value of $F$ would be unchanged but the the intercept related to the phase of the oscilltion will change. In addition, the first Landau level would be at 20 T not 30 T.

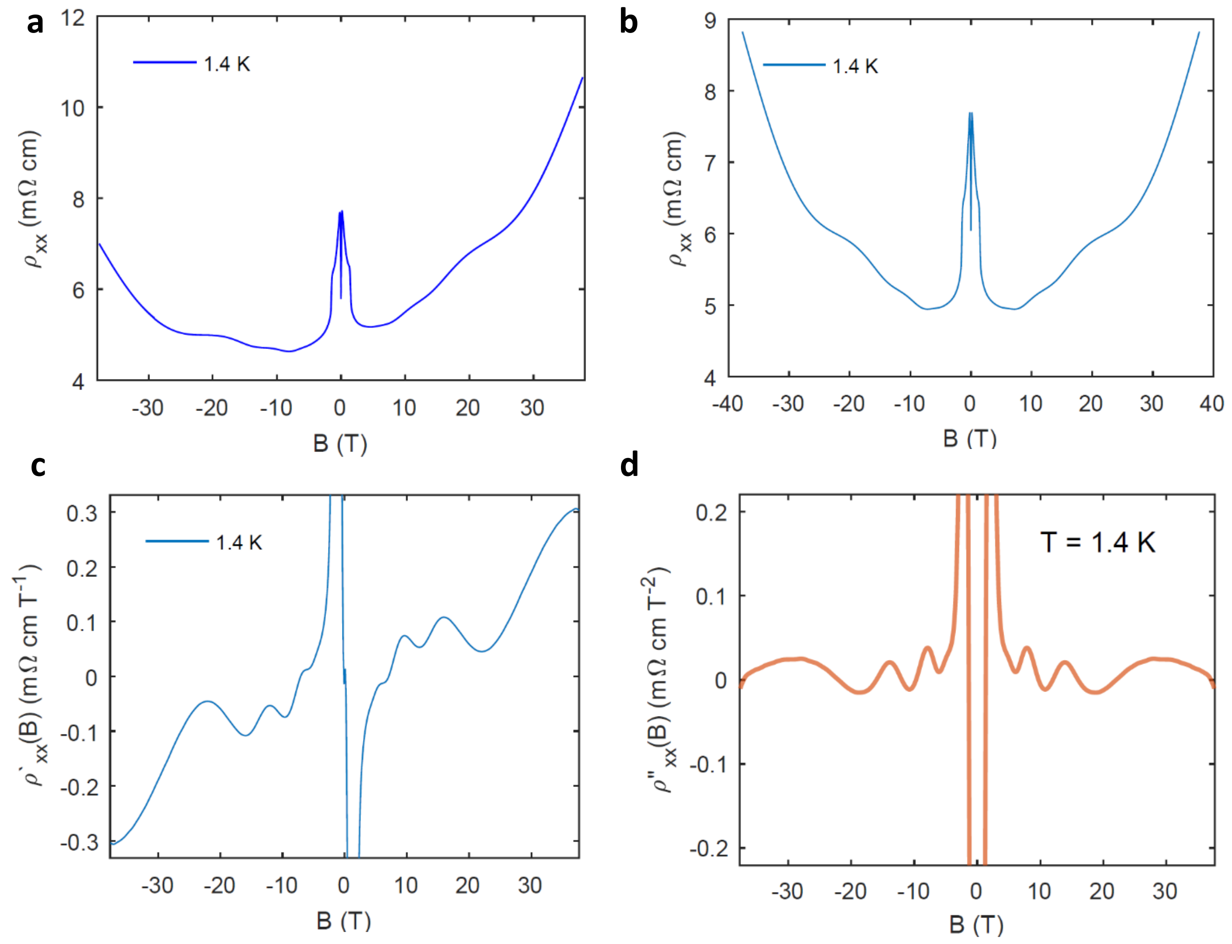


**Figure S5a–d . Shubnikov–de Haas oscillations in magnetotransport data measured up to 37 T. a** In-plane resistivity, $\rho_{xx}$(B), as function of magnetic field at 1.4 K with **B||c. b** Symmetrised data. By plotting the **c** first and **d** second derivatives with respect to B, namely $\rho'_{xx}$(B) and $\rho''_{xx}$(B), we are clearly able to observe the peaks and valleys of the quantum oscillations.

Figure S6a shows the raw in-plane resistivity data obtained from the 45 T Bitter magnet at the NHMFL at 1.7 K and 2.8 K with B||c. We augment the high-field (11 T < B < 45 T) data with low-field (–13 T < B < 13 T) measurements performed on a 14 T PPMS (Quantum Design). In the same way, we plot the first derivative of $\rho_{xx}$(B), in Figures S6b and c.

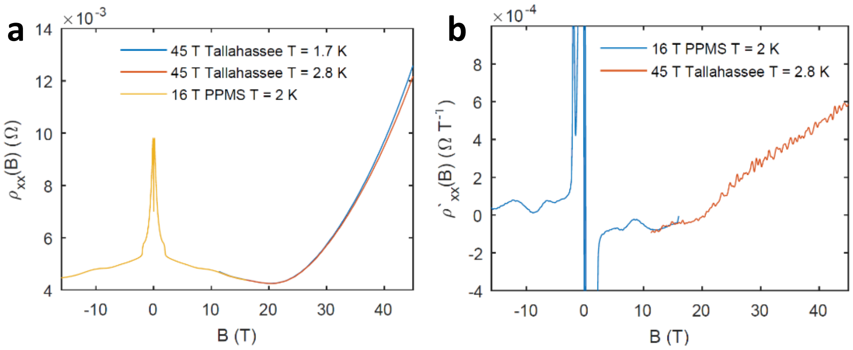


**Figure S6. Magnetotransport data measured up to 45 T. a**, In-plane resistivity, $\rho_{xx}$(B), as a function of magnetic field with **B||c** measured at T = 1.7 K and T = 2.8 K for 11 T < B < 45 T and T = 2 K for –16 T < B < 16 T. **b,** The first derivative of $\rho_{xx}$(B) with respect to B.

SdH oscillations in the resistivity of the flux-grown ECA crystals was observed across numerous samples. The frequency of these oscillations are listed in Table S2. As there is only 1 period of oscillation for measurements below 16 T, there is a larger uncertainty in the estimate of the oscillation frequency obtained in the data up to 16 T compared to that which is obtained in the data up to 37 T. Nonetheless, the estimated frequencies from the different instruments are consistent within the experimental errors.

| Sample | Frequency (T) | Remarks |
|---|---|---|
| DF2 | 25 (3) | Nijmegen measured to 37 T |
| DF2 | 23.7 | 16 T PPMS |
| CD13 | 23 (2) | 16 T PPMS |
| BQ1 | 23 (5) | 16 T PPMS |
| CL1 | 21 (5) | 16 T PPMS |
| CQ1 | 22 (4) | 16 T PPMS |
| CQ5 | 20 (7) | 16 T PPMS |
| CQ7 | 19 (5) | 16 T PPMS |
| | | |

**Table S2.** Frequency of SdH oscillations measured on different ECA crystals from the same batch.

# 3. DFT Calculations

To compute the electronic band structure, we used lattice parameters for $T < T_N$ in the DFT calculation. Computational details are provided in the main text. We estimate that the measured lattice parameters at 300 K, which are $a$ = 0.4442 nm and $c$ = 0.7331 nm, change to $a$ = 0.443 nm and $c$ = 0.729 nm at 10 K. This estimation of the change is based on the powder neutron diffraction work by May *et al.* on $AZn_2Sb_2$ ($A$ = Ca, Yb)[7], which is isostructural to $EuCd_2As_2$. In $AZn_2Sb_2$, the $a$ and $c$ lattice parameters decreased by 0.2 % and 0.5 % respectively when the sample was cooled from 300 K to 10 K.

We find that changing the $a$ lattice parameter from its low temperature value of 0.443 nm to 0.445 nm at fixed $c$ = 0.729 nm does not shift the Weyl node along $k_z$ or change the curvature of the bands in the vicinity of $E_F$. Changing $c$ from 0.729 nm to 0.735 nm at fixed $a$ = 0.445 nm causes a 4% shift in the Weyl node along $k_z$. These results demonstrate that the predictions are robust to within reasonable uncertainties in the lattice parameters.

The calculated band structure along the M-Γ-A high symmetry line with the ground state magnetic structure (A-type anti-ferromagnetic order with in-plane Eu moments) is shown in Figure S7a. The band structure presents a small direct gap at Γ. To check the robustness of this result, we have also calculated the band structure with the same magnetic order but varying the lattice constant from 0.729 nm to 0.735 nm in steps of 0.1 nm. In all cases we obtained very similar band structures, all gapped at the Fermi level.

We next computed the band structure for the case where the Eu moments are fully aligned along the c-axis, shown in Figure S7b. In this case, the gap is closed and two Weyl points appear at $k_0 = 0.26\ nm^{-1}$, which is around 6% of the Γ-A distance. Since the parent AFM band structure was insulating, and there are no other Fermi pockets present, by electron counting the Weyl points appear exactly at the Fermi level. To confirm these are Weyl points we also computed the in-plane dispersion when $k_z=k_0$, which is shown in Figure S8 and confirms the

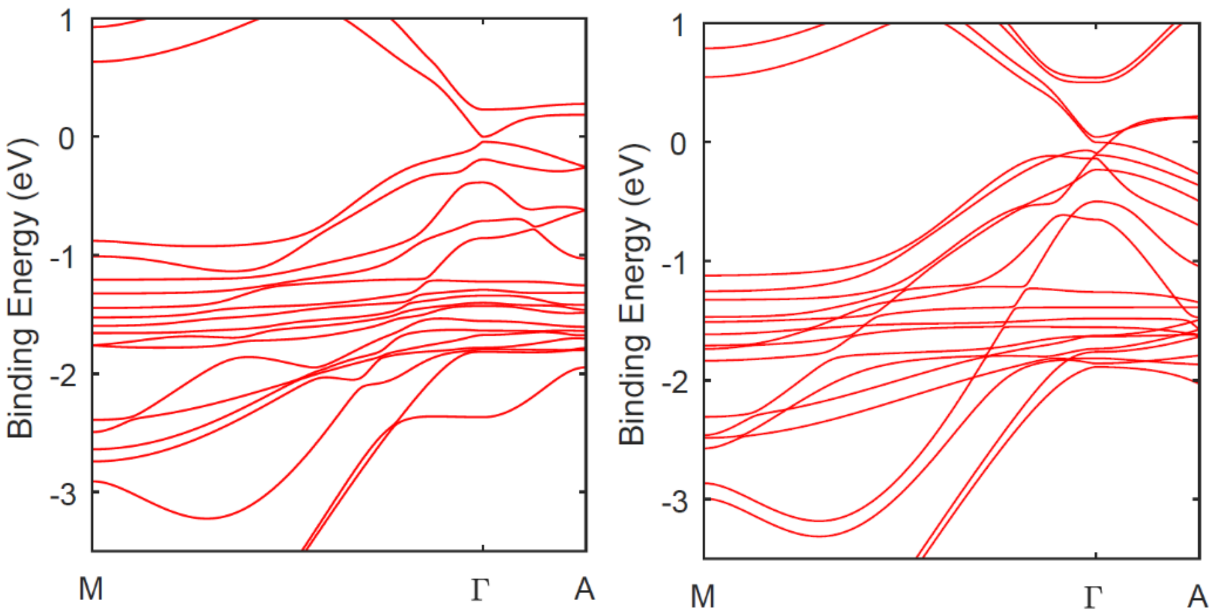


**Figure S7. The calculated electronic band structure for ECA. a,** The calculated electronic band structure for ECA for the ground state magnetic structure displays an avoided band crossing at the Γ point. **b**, This gap is closed when the moments are fully aligned along the c-axis at a point along the Γ-A high symmetry line.

point-like nature of the degeneracy and its in-plane linear dispersion. Since inversion symmetry is preserved in the ferromagnetic state, the Weyl points at opposite values of $k_z$ must have opposite Chern numbers.

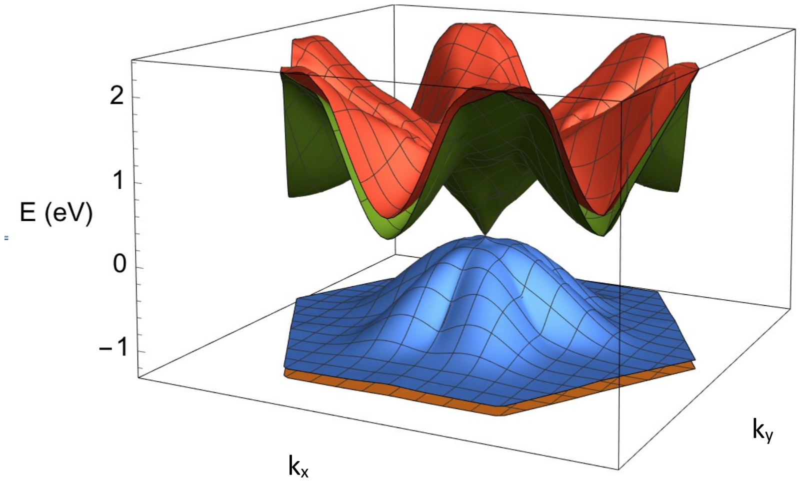


**Figure S8. The in-plane dispersion of the Weyl node. a,** The DFT calculated in-plane electronic structure of the 4 bands that are closest to the chemical potential in the ferromagnetic state with $k_z$=$k_0$.

To further characterize the Weyl nodes, we developed a low-energy two-band model constrained by symmetry. In the presence of a magnetic field in the *z* direction, the point group $D_{3d}$ reduces to $S_6$ where the $C_{2x}$ rotation and the mirror $M_x$ are broken, while inversion $I$ and the $C_{3z}$ and $S_6$ rotations are preserved. In addition, time-reversal symmetry $T$ is also broken, but the combinations $TC_{2x}$ and $TM_x$ are preserved. The Weyl points in the presence of the field are located in the Γ−A line, where the little group is just $C_3$. However, the operation $TC_{2x}$ leaves $k_z$ invariant and also constrains the Hamiltonian near the Weyl point. Taking $T = i\sigma_y$, $C_{2x} = i\sigma_x$, the effective Hamiltonian when $q$ is measured with respect to the node is,

$$H_{node}(q) = v_t q_z + v_\perp \sigma_z q_z + v_\parallel(\sigma_x q_x + \sigma_y q_y) + A_\perp q_z^2 + A_\parallel q_\parallel^2 + B_\parallel q_\parallel^4 + A_{TW}(\sigma_x 2 q_x q_y + \sigma_y(q_x^2 - q_y^2)),$$

where $q_\parallel^2 = q_x^2 + q_y^2$. Note that to fit the hole states accurately in the in-plane dispersion a fourth order term in momentum $B_\parallel$ was required. To obtain the parameters of this model we computed high-resolution cuts of the band structure in the directions Γ-K, Γ-M and Γ-A and fitted the results to the low energy model. The obtained parameters are shown in Table S3. The fits are overlaid the *ab-initio* calculations in Figure S9.

Due to the presence of the trigonal warping term $A_{TW}$ the Fermi surface has a small anisotropy of symmetry sin $3\theta$. To first order in $A_{TW}$ the correction to the energy vanishes in the x direction (Γ-K). Therefore, angular-averaged quantities like the Fermi velocity and effective mass are equivalent to those computed along the x direction to first order. Within this approximation, we estimate that the Fermi level required to obtain an in-plane Fermi momentum of $k_F$=0.28 nm$^{-1}$ is $E_F$ = - 52 meV. This is consistent with the estimated shift of 50 meV derived from ARPES. The Fermi velocity, defined as the slope at the Fermi level, is given by $v_F$ = -0.11 eV nm, from which we estimate an effective cyclotron mass $m_c^*$ = 0.18$m_e$, which is slightly larger than twice the one derived by fitting the decay of quantum oscillations to the LK formula.

| $v_t$(eV nm) | $v_\perp$(eV nm) | $v_\parallel$(eV nm) | $A_\perp$(eV nm$^2$) | $A_\parallel$(eV nm$^2$) | $B_\parallel$(eV nm$^4$) | $A_{TW}$ (eV nm$^2$) |
|---|---|---|---|---|---|---|
| 0.16 | 0.20 | 0.30 | -0.09 | 0.47 | -0.69 | 0.03 |

**Table S3. Parameters of the low energy model.**

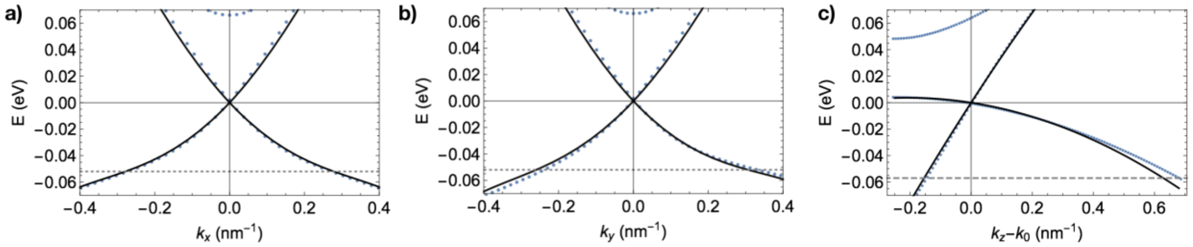


**Figure S9. Low energy dispersion near the Weyl point.** Energies computed from *ab-initio* are shown as dots, and the low-energy model fit is shown as a full line. **a**, In-plane dispersion along the x direction (Γ-K). **b**, Dispersion in the y direction (Γ-M). **c**, Dispersion in the z direction (Γ-A). The horizontal dashed line is the chemical potential that gives an in-plane Fermi momentum of 0.28 nm$^{-1}$ as obtained from quantum oscillations.

# 4. Low field magnetotransport

Low field magnetotransport measurements were performed by a five-probe method on a 14 T PPMS (Quantum Design) with **B**||**c**. The crystal was shaped into a Hall bar with dimensions of 0.91x0.33x0.056 $mm^3$. Figures S10a–d show the symmetrized in-plane longitudinal and Hall resistivities, $\rho_{xx}$ and $\rho_{yx}$, at various temperatures above and below $T_N$. Below $T_N$, the longitudinal resistivity peaks in an applied field of ~ 0.2 T and decreases at higher field strengths, as shown in **a**. The resistivity peak increases with temperature up to $T_N$ and is then suppressed at higher temperatures as shown in Figure S10c. This is in agreement with earlier magnetotransport studies of ECA[3]. Above $T_N$, the Hall resistivity increases linearly with applied field as shown in Figure S10d. As the sample is cooled below $T_N$, an anomalous feature (-2 T < B < 2 T) above the linear background develops as shown in Figure S10b**.** This deviation from the linear background is most pronounced at $\pm$0.2 T.

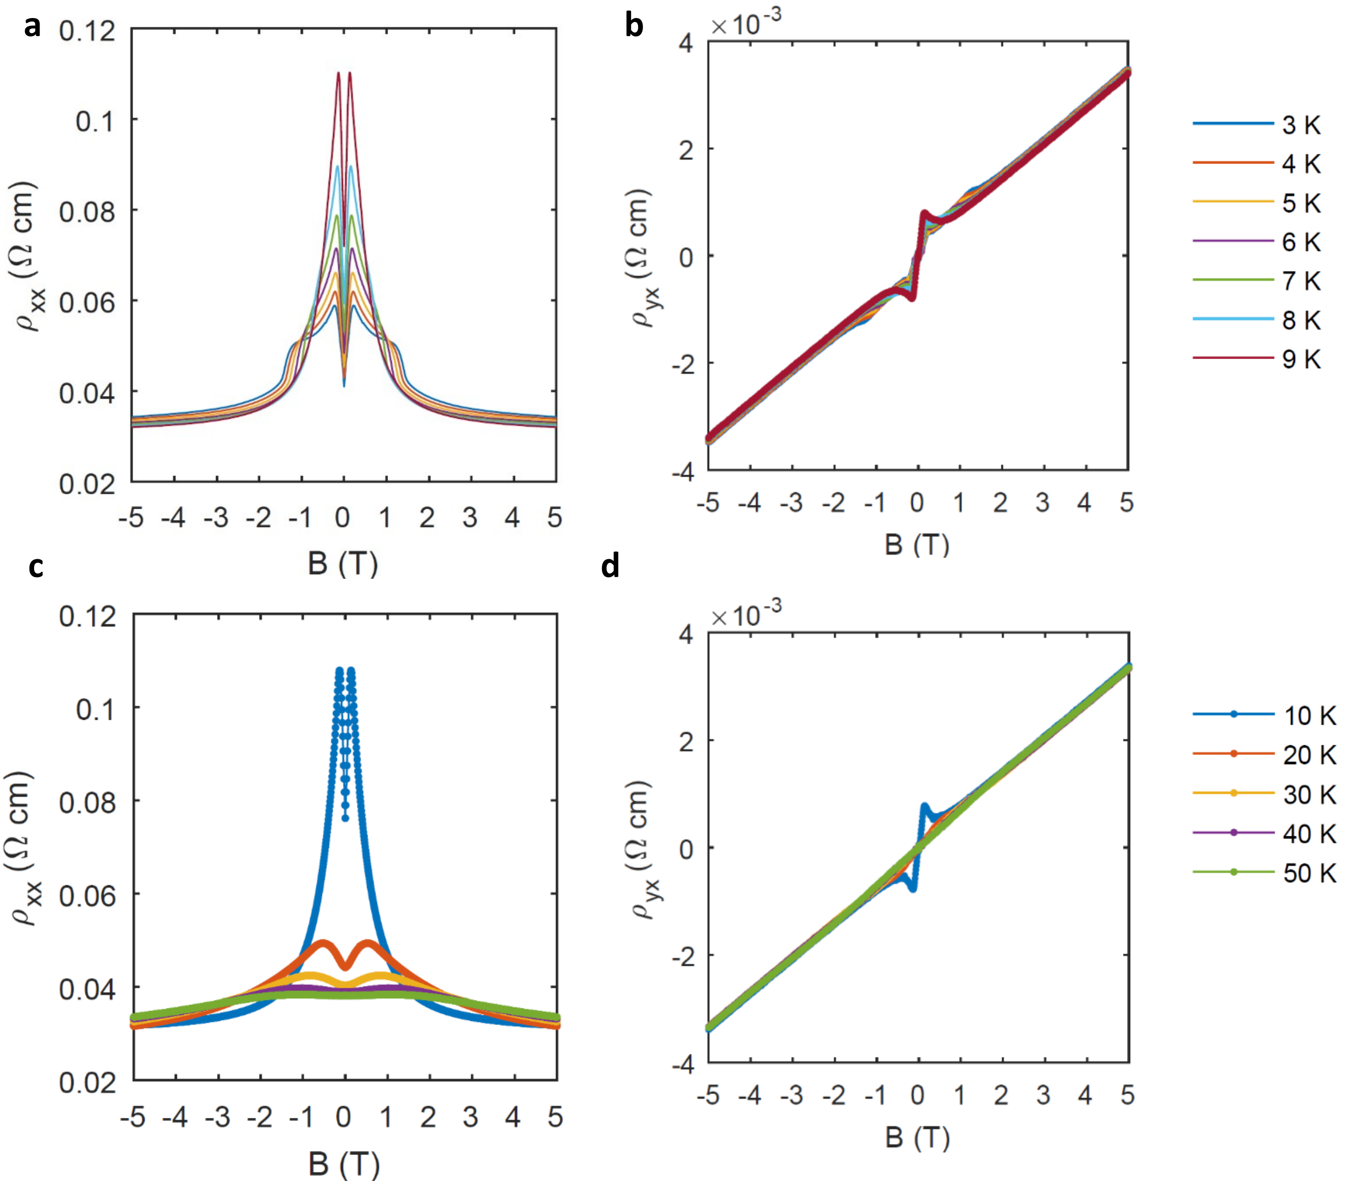


**Figure S10a–d. Longitudinal and Hall resistivity of ECA at various temperatures. a, c** The longitudinal resistivity at various temperatures below and above $T_N$ respectively. **b, d** Similarly for the Hall resistivity.

The in-plane conductivity, $\sigma_{yx}(\mathrm{B})$, obtained by inverting the resistivity matrix is given by,

$$\sigma_{yx} = \frac{-\rho_{yx}}{{\rho_{yx}}^2 + {\rho_{xx}}^2},$$

and is shown in Figure S11a. In the measured field range with B>B$_c$, $\rho_{xx}(\mathrm{B})$ is approximately constant (Fig. S5b) and $\rho_{yx} \ll \rho_{xx}$. Therefore the normal part of $\sigma_{yx}$ is approximately linear in B. Given this, a linear background was subtracted from $\sigma_{yx}(\mathrm{B})$ to give $\sigma_{\mathrm{yx}}^{\mathrm{AHE}}(\mathrm{B})$ in Figure S11c.

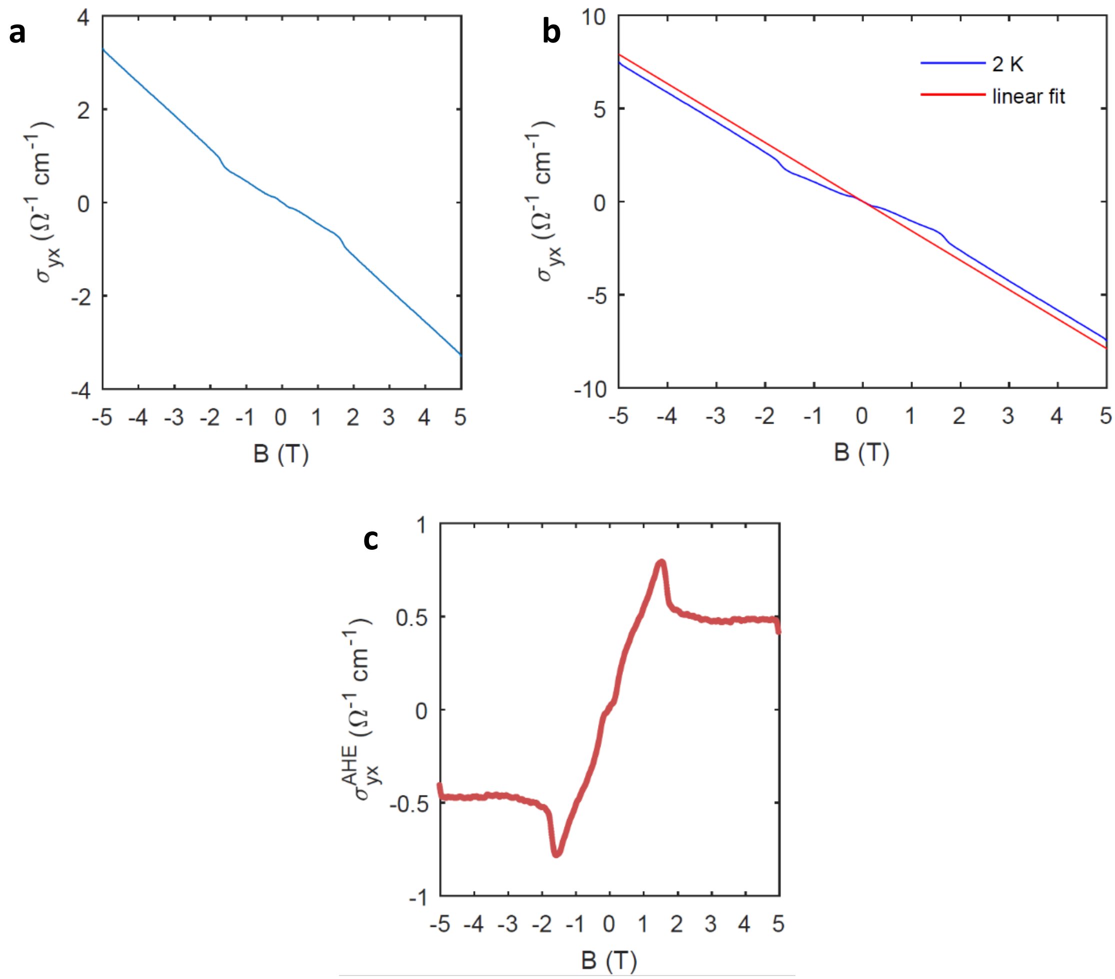


**Figure S11a - c. a**, The in-plane Hall conductivity of ECA is obtained by inverting the resistivity matrix. **b**, An anomalous component to the Hall conductivity above the linear background ( in red) is saturated above the coercive field (B>B$_c$). **c**, the anomalous component of the Hall conductivity is obtained by subtracting $\sigma_{yx}(B)$, with the linear background.

# References

[1] Artmann, A., Mewis, A., Roepke, M. & Michels, G. *$AM_2X_2$* Compounds with the $CaAl_2Si_2$-Type Structure. XI. Structure and Properties of *$ACd_2X_2$ (A:* Eu, Yb; *X:* P, As, Sb). *Z. Anorg. Allg. Chem.* **622**, 679 (1996).

[2] Schellenberg, I., Pfannenschmidt, U., Eul, M., Schwickert, C. & Pöttgen, R. A 121Sb and 151Eu Mössbauer Spectroscopic Investigation of $EuCd_2X_2$ (*X* =P, As, Sb) and $YbCd_2Sb_2$. *Z. Anorg. Allg. Chem.* **637**, 1863 (2011).

[3] Rahn, M. C. *et al*. Coupling of magnetic order and charge transport in the candidate Dirac semimetal $EuCd_2As_2$. *Phys. Rev. B* **97**, 214422 (2018).

[4] Wang, H. P., Wu, D. S., Shi, Y. G. & Wang, N. L. Anisotropic transport and optical spectroscopy study on antiferromagnetic triangular lattice $EuCd_2As_2$: An interplay between magnetism and charge transport properties. *Phys. Rev. B* **94**, 045112 (2016).

[5] A. A. Coelho, *TOPAS Academic Version 5*. Coelho Software: Brisbane, Australia, 2012.

[6] Wang, C. M., Lu, H.-Z. & Shen, S.-Q. Anomalous phase shift of quantum oscillations in 3D topological semimetals. Phys. Rev. Lett. **117**, 077201 (2016).

[7] May, A. F., *et al.* Properties of single crystalline $AZn_2Sb_2$ (A = Ca,Eu,Yb). *J. Appl. Phys.* **111**, 033708 (2012).
